# Supplementary material for: BNEM: A Boltzmann Sampler Based on Bootstrapped Noised Energy Matching
Source: arXiv:2409.09787 source file (2026-03-09)
Supplement: Supplementary file 1 [file endem_detail.tex]

\section{Training Details}\label{app:endem_train}
Algorithm \ref{alg:endem} describes NEM in detail. The key difference in training the BNEM is only in the inner-loop.

To train the BNEM, it's crucial that the bootstrap energy estimation at $t$ can be accurate only when the noised energy at $s$ is well-learned. Therefore, we need to sequentially learn energy at small t using the original
MC energy estimator then refines the estimator using bootstrap for large t, which is inefficient. To be more efficient, we adapt a rejection training scheme: (a) given $s$ and $t$, we first compute the loss of targeting the MC energy estimator (\ref{eq:mc-energy-estimator}), $l_s$ and $l_t$; (b) These losses indicate how does the energy network fit the noised energies at different times, and therefore compute $\alpha=l_s/l_t$ as an indicator; (c) with probability $\alpha$, we accept targeting a energy estimator bootstrapped from $s$ and otherwise we stick to target the original MC estimator. We provide a full description of the inner-loop of BNEM training in Algorithm \ref{alg:bendem}.
\input{algorithms/endem_alg}
\input{algorithms/bendem_alg}
